# Supplementary material for: Secrecy: Secure collaborative analytics on secret-shared data
Source: arXiv:2102.01048 source file (2022-02-03)
Supplement: Supplementary file 1 [file appendix.tex]

\section{Additional experimental results}

\subsection{Group-by operator logic}\label{sec:group_appendix}

The logic of oblivious group-by is given in Algorithm~\ref{alg:group}.
% and is based on the protocol in~\cite{DBLP:journals/iacr/JonssonKU11}.   
Let $a_k$ be the group-by key, $a_w$ the aggregated attribute, $a_g$ the extra attribute that stores the aggregation result (initialized with $a_w$), and $a_v$ the `valid' bit (same notation as in Section~\ref{sec:secure_operators}).  The first step is to sort the input relation on the group-by key (\textbf{line 1}). Then, the operator scans the sorted relation and, for each pair of adjacent tuples, applies an oblivious equality comparison on $a_k$  (\textbf{line 3}). The result of this comparison ($b$) is used to aggregate (\textbf{line 4}), set the `valid' bit (\textbf{line 5}), and ``mask'' (\textbf{line 6}) obliviously. Aggregation is updated incrementally based on the values of the last pair of tuples  (\textbf{line 4}). \texttt{MIN}, \texttt{MAX}, \texttt{COUNT}, and \texttt{SUM} can be easily evaluated this way but for \text{AVG} we need to keep the sum (numerator) and count (denominator) separate.
When the scan is over, the algorithm requires a final shuffling  (\textbf{line 7}) to hide the group ``traces'' in case the relation (or a part of it) is opened to the learner; this step is only needed if no subsequent sorting is required in the query plan, which would obliviously re-order $R$ anyway.

\begin{algorithm}[t]
\small
%\Input{A stream $S$ of logs and a window $[t_s,t_e]$;}
%\Output{The graph snapshot $G_{[t_s,t_e]}$;}

%\BlankLine

%\Comment{The sort direction does not matter}
sort input relation $R$ on $a_k$;

%let $a_k$ be the group-by key, $a_w$ the aggregated attribute, and $a_g$ the extra attribute that stores the aggregation result;

\For {each pair of adjacent tuples ($t_i$, $t_{i+1}$), $0\leq i < |R|$,} {
  
  \Comment{Are tuples in the same group?}
  
  let $b \leftarrow t_i[a_k] \stackrel{?}{=} t_{i+1}[a_k]$;
  
  \Comment{Aggregation}
  
  $t_{i+1}[a_g] \leftarrow b\cdot agg\Big(t_i[a_g], t_{i+1}[a_g]\Big) + (1-b)\cdot t_{i+1}[a_g]$;
  
  $t_{i}[a_v] \leftarrow \lnot b$;
  
  \Comment{Masking}
  $t_i \leftarrow b* t_{inv}~~+~~(1-b)* t_i$;
  
%  \For {each attribute $a\neq a_v$ of $t_i$} {
%  	
%	let $r$ be an invalid value;
%	
%  	$a \leftarrow b\cdot r~~+~~(1-b)\cdot a$;
%  } 
  }
  shuffle R; %\Com{Only if there is no subsequent order-by}

%re-distribute $E_h$ based on $(id_{src},id_{dst},id_{corr})$;
%Pair up half edges in each partition and create the set $E_{comm}$ of edges for communication activities;
%\textbf{return} $E_w \cup E_{c}$
\caption{\small Main control-flow of oblivious group-by}\label{alg:group}
\end{algorithm}

Distinct is a special case of group-by where  $a_k$ is in this case the distinct attribute. As such, it follows a slightly different version of Alg.~\ref{alg:group} where, for each pair of adjacent tuples, we apply the equality comparison on $a_k$ (\textbf{line 3}) and set the distinct bit $t_{i+1}[a_v]$ to $\lnot b$ (the value $t_0[a_v]$ of the first tuple is set to 1).
Lines \textbf{4-7} are simply omitted in this case because distinct does not require aggregation, masking or shuffling.
All equality comparisons (\textbf{line 3}) within the loop can be performed \emph{in bulk} for all pairs of tuples.

\subsection{Comparison with other MPC frameworks}\label{sec:eval_comparison}

In this section, we compare \ours with two state-of-the-art MPC frameworks: SMCQL~\cite{Bater2017SMCQL} and the 2-party semi-honest version of EMP~\cite{emp-toolkit}. We choose SMCQL (the ORAM-based version) as the only open-source relational framework with a semi-honest model and no information leakage (cf.~Table~\ref{tbl:comparison}). More recent systems, such as Shrinkwrap~\cite{bater2018shrinkwrap}, SAQE~\cite{bater2020saqe}, and a new version of SMCQL, although not publicly available, build on top of EMP. 
%We choose EMP as it is the basis of many relational frameworks that are not publicly available, including a new (faster) version of SMCQL, and 
Senate (which is also not publicly available) relies on EMP as well, albeit its malicious version \cite{Poddar2021Senate}.
We stress that these systems use MPC protocols that rely on different threat models and thus are not directly comparable.
The purpose of these experiments is to showcase the end-to-end performance of the actual implementations for relational MPC and not to compare the underlying protocols.

\stitle{Comparison with SMCQL.} In the first set of experiments, we aim to reproduce the results presented in the SMCQL paper (Figure 7)~\cite{Bater2017SMCQL} on our experimental setup. We run the three medical queries on SMCQL and \ours, using a sample of $25$ tuples per data owner (50 in total), and present the results in Table~\ref{tab:smcql-results}. We use the plans and default configuration of protected and public attributes, as in the SMCQL project repository~\cite{smcql-repository}. %\footnote{\url{https://github.com/smcql/smcql}}. 
As we can see, \ours is over $2000\times$ faster than SMCQL in all queries, even though SMCQL pushes operators outside the MPC boundary by allowing data owners to execute part of the computation on their plaintext data. In the SMCQL experiment, each computing party is also a data owner and, although it provides $25$ tuples per relation to a query, only $8$ of those enter the oblivious part of the plan; the rest are filtered out before entering the MPC circuit.

\stitle{Comparison with EMP.} EMP is a general-purpose MPC framework and does not provide implementations of relational operators out-of-the-box. 
For this set of experiments, we implemented an equi-join operator using the sample program available in the SoK project~\cite{sok-project} %\footnote{https://github.com/MPC-SoK/frameworks/blob/master/emp/sh\_test/test/xtabs.cpp} 
and we also use the oblivious sort primitive provided in the EMP repository~\cite{emp-toolkit}. %\footnote{https://github.com/emp-toolkit/emp-sh2pc}.
%We compare \ours with EMP on two relational operators: an equi-join\footnote{https://github.com/MPC-SoK/frameworks/blob/master/emp/sh\_test/test/xtabs.cpp} and an oblivious sort\footnote{https://github.com/emp-toolkit/emp-sh2pc/blob/master/test/example.cpp}. These are the only two publicly available implementations of relational operators we could find. 
Figure~\ref{fig:emp-results} presents the results.
%, these were the only publicly available operator implementations we found. 
For joins, we use inputs of the same cardinality ($n=m$) and increase the size from $10K$ to $100K$ rows per input. We cap the time of these experiments to $15h$. Within the experiment duration, EMP can evaluate joins on up to $40K$ rows per input (in $14.3h$). \ours is $7.53\times$ faster for the same input size and can process up to $100K$ rows per input in a bit less than $12h$. %In addition, for joins on $40K$ rows per input, \ours has $7.53\times$ lower execution time than EMP. 
%In fact, \ours can process $100K$ rows per input in less time ($12h$) than the time EMP needs to process $40K$ rows per input ($14.3h$). 
The performance gap between \ours and EMP on oblivious sort is less dramatic but still considerable. In this case, both frameworks scale to much larger inputs and \ours is up to $1.45\times$ faster ($3.27h$ vs $4.74h$ for $4M$ input~rows). 

\begin{figure}[t]
    \centering
        \begin{minipage}{.24\textwidth}
            \begin{subfigure}{\textwidth}
            \centering
  		\includegraphics[width=\linewidth]{figs/experiments/emp-join-sysx.png}
 			 %\vspace{-6mm}
			%\caption{Join.}\label{fig:emp-join}
            \end{subfigure}
        \end{minipage}
        \hfill
        \begin{minipage}{.23\textwidth}
            \begin{subfigure}{\textwidth}
            \centering
  			\includegraphics[width=\linewidth]{figs/experiments/emp-sort-sysx.png}
            \vspace{-5mm}
         %\caption{Sort.}\label{fig:emp-sort}
            \end{subfigure}
        \end{minipage}
         %\vspace{-2mm}
         \caption{Performance comparison between EMP and \ours}
        	\label{fig:emp-results}
        	%\vspace{-3mm}
\end{figure}

\begin{table}[t]
\scriptsize
\centering
\begin{tabular}{c|r|r|r|}
\cline{2-4}
\multicolumn{1}{l|}{} &
  \multicolumn{1}{c|}{\textbf{Comorbidity}} &
  \multicolumn{1}{c|}{\textbf{Recurrent C. Diff.}} &
  \multicolumn{1}{c|}{\textbf{Aspirin Count}} \\ \hline
  \hline
\multicolumn{1}{|c|}{\textbf{SMCQL}} &
$197s$& $804s$ & $796s$\\ \hline
\multicolumn{1}{|c|}{\textbf{\ours}} &
$0.083s$& $0.092s$ & $0.171s$\\ \hline
\bottomrule
\end{tabular}
\caption{SMCQL and \ours execution times for the three medical queries from~\cite{Bater2017SMCQL} on 25 tuples per input relation.}
\label{tab:smcql-results}\vspace{-3mm}
\end{table}\vspace{25mm}

\subsection{Queries}
\label{app:queries}

Here we list the queries used in Section~\ref{sec:evaluation} (in SQL syntax):

\stitle{Comorbidity}:

{\small 
\texttt{SELECT diag, COUNT(*) cnt}

\texttt{FROM diagnosis}

\texttt{WHERE pid IN cdiff\_cohort}

\texttt{GROUP BY diag}

\texttt{ORDER BY cnt DESC}

\texttt{LIMIT 10}
}\vspace{1mm}

\stitle{Recurrent C. Diff.}:

{\small
\texttt{WITH rcd AS (}

\hspace{5mm}\texttt{SELECT pid, time, row\_no() OVER}
        
\hspace{5mm}\texttt{(PARTITION BY pid ORDER BY time)}

\hspace{5mm}\texttt{FROM diagnosis}
    
\hspace{5mm}\texttt{WHERE diag=cdiff)}

\hspace{2mm}\texttt{SELECT DISTINCT pid}

\hspace{2mm}\texttt{FROM rcd r1 JOIN rcd r2 ON r1.pid = r2.pid} 

\hspace{2mm}\texttt{WHERE r2.time - r1.time >= 15 DAYS}

\hspace{2mm}\texttt{AND r2.time - r1.time <= 56 DAYS}

\hspace{2mm}\texttt{AND r2.row\_no = r1.row\_no + 1}
}\vspace{1mm}

\stitle{Aspririn Count}:

{\small 

\texttt{SELECT count(DISTINCT pid)}

\texttt{FROM diagnosis as d, medication as m on}

 \texttt{d.pid = m.pid}
 
\texttt{WHERE d.diag = hd AND m.med = aspirin}

\texttt{AND d.time <= m.time}
}\vspace{1mm}

\stitle{Password Reuse}:

{\small 

\texttt{SELECT ID}

\texttt{FROM R}

\texttt{GROUP BY CONCAT(ID, PWD)}

\texttt{HAVING COUNT(*)>1}
}\vspace{1mm}

\stitle{Credit Score}:

{\small 

\texttt{SELECT S.ID}

\texttt{FROM (}

\hspace{2mm}\texttt{SELECT ID, MIN(CS) as cs1, MAX(CS) as cs2}

\hspace{2mm}\texttt{FROM R}
 
\hspace{2mm}\texttt{WHERE R.year=2019}

\hspace{2mm}\texttt{GROUP-BY ID ) as S}

\texttt{WHERE S.cs2 - S.cs1 > c}
}\vspace{2mm}

The three TPC-H queries (\textbf{Q4}, \textbf{Q6}, \textbf{Q13}) we used can be found in the benchmark specification~\cite{tpch}.
